# Supplementary material for: $\alpha$-approximate Reductions: a Novel Source of Heuristics for Better Approximation Algorithms
Source: arXiv:2106.14169 source file (2021-06-27)
Supplement: Supplementary file 1 [file appendix.tex]

\section*{Appendix}

The last column denotes the improvement ($\texttt{imprv}$) in the solution quality. It is defined as $(\texttt{AA}(G) - \texttt{LA}(G)) \times 100 / \texttt{EX}(G)$ for $G$ for which $\texttt{AA}(G) > \texttt{LA}(G)$.

\begin{center}
\begin{table}
\centering
\begin{tabular}{|c|c|c|c|c|c|c|}
\hline
ID	&	$|V(G)|$	&	$|E(G)|$	&	$\texttt{EX}(G)$	&	$\texttt{AA}(G)$	&	$\texttt{LA}(G)$	&	$\texttt{imprv}$ \\
\hline
1	&	1643	&	9857	&	194	&	254	&	238	&	8.25	\\
2	&	2919	&	14688	&	306	&	498	&	467	&	10.13	\\
3	&	4251	&	25662	&	329	&	669	&	616	&	16.11	\\
4	&	7753	&	61939	&	365	&	1021	&	924	&	26.58	\\
5	&	8469	&	68036	&	376	&	1114	&	1016	&	26.06	\\
6	&	2407	&	9728	&	308	&	464	&	454	&	3.25	\\
7	&	4554	&	27319	&	342	&	719	&	660	&	17.25	\\
8	&	3951	&	11838	&	471	&	862	&	969	&	--	\\
9	&	3750	&	14945	&	395	&	730	&	744	&	--	\\
10	&	8963	&	44486	&	513	&	1541	&	1559	&	--	\\
11	&	9471	&	37693	&	565	&	1831	&	1918	&	--	\\
12	&	7796	&	38975	&	474	&	1324	&	1339	&	--	\\
13	&	7659	&	22775	&	629	&	1672	&	1907	&	--	\\
14	&	8903	&	26668	&	649	&	1930	&	2179	&	--	\\
15	&	6412	&	31779	&	443	&	1094	&	1114	&	--	\\
16	&	4888	&	19664	&	436	&	935	&	969	&	--	\\
17	&	7406	&	59503	&	353	&	961	&	885	&	21.53	\\
18	&	6411	&	50982	&	332	&	842	&	789	&	15.96	\\
19	&	5605	&	50589	&	294	&	670	&	616	&	18.37	\\
20	&	5722	&	34395	&	375	&	883	&	818	&	17.33	\\
21	&	2007	&	14043	&	195	&	295	&	274	&	10.77	\\
22	&	6508	&	26088	&	484	&	1232	&	1316	&	--	\\
23	&	1711	&	5094	&	314	&	387	&	412	&	--	\\
24	&	3743	&	26187	&	277	&	529	&	489	&	14.44	\\
25	&	3856	&	15487	&	391	&	749	&	808	&	--	\\
26	&	8527	&	76860	&	345	&	1045	&	978	&	19.42	\\
27	&	3004	&	9196	&	415	&	651	&	694	&	--	\\
28	&	6615	&	26469	&	496	&	1265	&	1324	&	--	\\
29	&	4194	&	29070	&	299	&	610	&	542	&	22.74	\\
30	&	9545	&	85862	&	376	&	1168	&	1081	&	23.14	\\
31	&	5647	&	45093	&	309	&	745	&	684	&	19.74	\\
32	&	1818	&	12777	&	185	&	265	&	249	&	8.65	\\
33	&	2526	&	7473	&	387	&	564	&	612	&	--	\\
34	&	2606	&	18526	&	224	&	374	&	352	&	9.82	\\
35	&	2829	&	14140	&	301	&	479	&	444	&	11.63	\\
36	&	6114	&	36656	&	391	&	955	&	900	&	14.07	\\
37	&	3658	&	32922	&	232	&	447	&	412	&	15.09	\\
38	&	6170	&	36791	&	400	&	967	&	903	&	16.00	\\
39	&	4469	&	26995	&	332	&	704	&	633	&	21.39	\\
40	&	2913	&	8921	&	405	&	625	&	680	&	--	\\
41	&	9145	&	27568	&	654	&	1964	&	2260	&	--	\\
42	&	1741	&	8830	&	223	&	287	&	282	&	2.24	\\
43	&	5304	&	31902	&	365	&	826	&	766	&	16.44	\\
44	&	3908	&	19475	&	358	&	666	&	669	&	--	\\
45	&	1521	&	13548	&	134	&	185	&	178	&	5.22	\\
46	&	7880	&	39297	&	476	&	1352	&	1369	&	--	\\
47	&	7709	&	23177	&	621	&	1665	&	1905	&	--	\\
48	&	9642	&	76876	&	403	&	1268	&	1162	&	26.30	\\
49	&	7847	&	39357	&	477	&	1341	&	1354	&	--	\\
50	&	4645	&	32619	&	312	&	657	&	605	&	16.67	\\
\hline
\end{tabular}
\caption{Small Erdos Renyi  Graphs.  \label{table:erdos-renyi-small-1}}
\end{table}
\end{center}

\begin{center}
\begin{table}
\centering
\begin{tabular}{|c|c|c|c|c|c|c|}
\hline
ID 	&	$|V(G)|$	&	$|E(G)|$	&	$\texttt{EX}(G)$	&	$\texttt{AA}(G)$	&	$\texttt{LA}(G)$	&	$\texttt{iprv}$ \\
\hline
51	&	8002	&	72289	&	342	&	978	&	901	&	22.51	\\
52	&	1709	&	6819	&	256	&	330	&	322	&	3.13	\\
53	&	3614	&	25459	&	270	&	511	&	474	&	13.70	\\
54	&	8467	&	76198	&	349	&	1048	&	956	&	26.36	\\
55	&	8500	&	59481	&	404	&	1222	&	1117	&	25.99	\\
56	&	6828	&	27402	&	495	&	1321	&	1369	&	--	\\
57	&	2533	&	15162	&	251	&	407	&	366	&	16.33	\\
58	&	9107	&	45596	&	490	&	1561	&	1546	&	3.06	\\
59	&	9413	&	37565	&	567	&	1810	&	1889	&	--	\\
60	&	4777	&	43015	&	268	&	591	&	544	&	17.54	\\
61	&	6639	&	53085	&	331	&	888	&	796	&	27.79	\\
62	&	4819	&	24444	&	380	&	833	&	821	&	3.16	\\
63	&	5410	&	32760	&	368	&	838	&	773	&	17.66	\\
64	&	9556	&	28778	&	662	&	2054	&	2386	&	--	\\
65	&	1343	&	10564	&	130	&	176	&	166	&	7.69	\\
66	&	3428	&	13854	&	375	&	649	&	667	&	--	\\
67	&	4129	&	16524	&	414	&	815	&	854	&	--	\\
68	&	1546	&	10748	&	164	&	224	&	205	&	11.59	\\
69	&	8275	&	32828	&	542	&	1598	&	1690	&	--	\\
70	&	9767	&	77979	&	400	&	1300	&	1186	&	28.50	\\
71	&	4711	&	32790	&	314	&	669	&	612	&	18.15	\\
72	&	1943	&	7821	&	275	&	373	&	375	&	--	\\
73	&	4264	&	29628	&	305	&	612	&	547	&	21.31	\\
74	&	6638	&	26723	&	491	&	1277	&	1312	&	--	\\
75	&	4263	&	29762	&	300	&	620	&	542	&	26.00	\\
76	&	4481	&	26759	&	335	&	703	&	665	&	11.34	\\
77	&	9862	&	69213	&	429	&	1392	&	1265	&	29.60	\\
78	&	6921	&	27259	&	500	&	1329	&	1426	&	--	\\
79	&	9838	&	88617	&	378	&	1200	&	1103	&	25.66	\\
80	&	2957	&	23407	&	223	&	386	&	369	&	7.62	\\
81	&	4683	&	42190	&	261	&	580	&	533	&	18.01	\\
82	&	9710	&	67776	&	435	&	1376	&	1278	&	22.53	\\
83	&	3336	&	23169	&	262	&	475	&	450	&	9.54	\\
84	&	2675	&	21663	&	212	&	339	&	330	&	4.25	\\
85	&	4714	&	42763	&	266	&	582	&	539	&	16.17	\\
86	&	7649	&	22960	&	627	&	1661	&	1867	&	--	\\
87	&	5207	&	15681	&	528	&	1129	&	1292	&	--	\\
88	&	5786	&	34578	&	384	&	909	&	867	&	10.94	\\
89	&	9136	&	27373	&	660	&	1988	&	2292	&	--	\\
90	&	6109	&	24556	&	469	&	1169	&	1231	&	--	\\
91	&	6331	&	44007	&	367	&	904	&	834	&	19.07	\\
92	&	3654	&	18226	&	344	&	633	&	635	&	--	\\
93	&	3751	&	15038	&	386	&	715	&	742	&	--	\\
94	&	8158	&	40792	&	474	&	1401	&	1405	&	--	\\
95	&	3429	&	20749	&	292	&	548	&	503	&	15.41	\\
96	&	4992	&	15041	&	512	&	1096	&	1250	&	--	\\
97	&	1825	&	7305	&	266	&	354	&	351	&	1.13	\\
98	&	1896	&	9483	&	237	&	324	&	305	&	8.02	\\
99	&	9897	&	69221	&	431	&	1438	&	1306	&	30.63	\\
100	&	7269	&	36180	&	465	&	1241	&	1257	&	--	\\
\hline
\end{tabular}
\caption{Small Erdos Renyi  Graphs. \label{table:erdos-renyi-small-2}}
\end{table}
\end{center}

%%%%%%% TABLE START %%%%%%%%%%%
\begin{center}
\begin{table}
\centering
\begin{tabular}{|c|c|c|c|c|c|c|}
\hline
ID 	&	$|V(G)|$	&	$|E(G)|$	&	$\texttt{EX}(G)$	&	$\texttt{AA}(G)$	&	$\texttt{LA}(G)$	&	$\texttt{iprv}$ \\
\hline
1	&	19804	&	138454	&	563	&	2794	&	2571	&	39.61	\\
2	&	12332	&	99128	&	457	&	1624	&	1474	&	32.82	\\
3	&	14212	&	56701	&	642	&	2728	&	2852	&	--	\\
4	&	20384	&	163573	&	559	&	2652	&	2459	&	34.53	\\
5	&	19676	&	78096	&	739	&	3761	&	3962	&	--	\\
6	&	13374	&	80081	&	518	&	2084	&	1946	&	26.64	\\
7	&	25714	&	232160	&	631	&	3141	&	2893	&	39.30	\\
8	&	15875	&	142662	&	464	&	1903	&	1812	&	19.61	\\
9	&	22932	&	137217	&	674	&	3585	&	3335	&	37.09	\\
10	&	14442	&	43448	&	773	&	3152	&	3579	&	--	\\
11	&	20382	&	81375	&	763	&	3925	&	4083	&	--	\\
12	&	27075	&	189663	&	724	&	3828	&	3524	&	41.99	\\
13	&	16941	&	50811	&	827	&	3710	&	4174	&	--	\\
14	&	25888	&	78013	&	1098	&	5629	&	6434	&	--	\\
15	&	21299	&	85344	&	781	&	4110	&	4263	&	--	\\
16	&	22554	&	135183	&	671	&	3473	&	3295	&	26.53	\\
17	&	23530	&	188371	&	632	&	3070	&	2822	&	39.24	\\
18	&	16680	&	116972	&	520	&	2381	&	2175	&	39.62	\\
19	&	13215	&	39531	&	757	&	2915	&	3271	&	--	\\
20	&	23604	&	165444	&	660	&	3347	&	3070	&	41.97	\\
21	&	14143	&	127141	&	441	&	1729	&	1600	&	29.25	\\
22	&	27967	&	223523	&	706	&	3702	&	3368	&	47.31	\\
23	&	13029	&	117220	&	433	&	1606	&	1459	&	33.95	\\
24	&	27186	&	81702	&	1153	&	5922	&	6700	&	--	\\
25	&	15996	&	144039	&	462	&	1951	&	1803	&	32.03	\\
26	&	13077	&	78569	&	511	&	2019	&	1896	&	24.07	\\
27	&	11888	&	71258	&	503	&	1876	&	1744	&	26.24	\\
28	&	14179	&	84866	&	521	&	2187	&	2072	&	22.07	\\
29	&	13255	&	79295	&	502	&	2067	&	1930	&	27.29	\\
30	&	21241	&	84897	&	776	&	4044	&	4269	&	--	\\
31	&	12293	&	85773	&	463	&	1761	&	1594	&	36.07	\\
32	&	17790	&	71326	&	695	&	3404	&	3566	&	--	\\
33	&	11402	&	45822	&	592	&	2167	&	2273	&	--	\\
34	&	13403	&	107597	&	455	&	1759	&	1609	&	32.97	\\
35	&	12405	&	73969	&	509	&	1940	&	1809	&	25.74	\\
36	&	26419	&	210619	&	674	&	3447	&	3166	&	41.69	\\
37	&	20395	&	183839	&	522	&	2459	&	2300	&	30.46	\\
38	&	22483	&	179759	&	596	&	2915	&	2719	&	32.89	\\
39	&	28222	&	225365	&	715	&	3682	&	3393	&	40.42	\\
40	&	10922	&	43727	&	595	&	2079	&	2191	&	--	\\
41	&	26331	&	158195	&	752	&	4064	&	3837	&	30.19	\\
42	&	13057	&	117399	&	430	&	1599	&	1479	&	27.91	\\
43	&	13319	&	93302	&	486	&	1887	&	1720	&	34.36	\\
44	&	13989	&	112372	&	468	&	1835	&	1705	&	27.78	\\
45	&	11100	&	77131	&	456	&	1597	&	1442	&	33.99	\\
46	&	22487	&	156926	&	634	&	3193	&	2936	&	40.54	\\
47	&	21608	&	108081	&	707	&	3699	&	3655	&	6.22	\\
48	&	14644	&	87898	&	542	&	2276	&	2141	&	24.91	\\
49	&	27629	&	165797	&	783	&	4284	&	4022	&	33.46	\\
50	&	11906	&	71354	&	509	&	1850	&	1767	&	16.31	\\

\hline
\end{tabular}
\caption{Medium Erdos Renyi  Graphs. \label{table:erdos-renyi-medium-1}
\end{table}
\end{center}
%%%%% TABLE ENDS %%%%%%%%%%%%%%

%%%%%%% TABLE START %%%%%%%%%%%
\begin{center}
\begin{table}
\centering
\begin{tabular}{|c|c|c|c|c|c|c|}
\hline
ID 	&	$|V(G)|$	&	$|E(G)|$	&	$\texttt{EX}(G)$	&	$\texttt{AA}(G)$	&	$\texttt{LA}(G)$	&	$\texttt{iprv}$ \\
\hline

\hline
\end{tabular}
\caption{Medium Erdos Renyi  Graphs. \label{table:erdos-renyi-medium-1}
\end{table}
\end{center}
%%%%% TABLE ENDS %%%%%%%%%%%%%%
